# Supplementary material for: CUBETESTERAI: Automated JUnit Test Generation using the LLaMA Model
Source: arXiv:2504.15286 source file (2025-03-13)
Supplement: Supplementary file 1 [file Appendix.tex]

% \appendix
% \chapter{Appendix}
% \label{appendix} 

% \newpage
% \section{JUnit Test Case Example}
